# Supplementary material for: Effect on Dark Matter Exclusion Limits from New Silicon Photoelectric Absorption Measurements
Source: arXiv:2010.15874 ancillary file (2021-07-05)
Supplement: Supplementary file 1 [file SupplMaterial.pdf]

# Effect on Dark Matter Exclusion Limits from New Silicon Photoelectric Absorption Measurements **Supplemental Material**

B. von Krosigk<sup>\*1</sup>, M.J. Wilson<sup>\*1,2</sup>, C. Stanford<sup>3,7</sup>, B. Cabrera<sup>3,8</sup>, R. Calkins<sup>4</sup>, D. Jardin<sup>4</sup>,  
N.A. Kurinsky<sup>5,9</sup>, F. Ponce<sup>3</sup>, and C.-P. Wu<sup>6</sup>

<sup>1</sup>*Institut für Experimentalphysik, Universität Hamburg, 22761 Hamburg, Germany*

<sup>2</sup>*Department of Physics, University of Toronto, Toronto, ON M5S 1A7, Canada*

<sup>3</sup>*Department of Physics, Stanford University, Stanford, CA 94305 USA*

<sup>4</sup>*Department of Physics, Southern Methodist University, Dallas, TX 75275, USA*

<sup>5</sup>*Fermi National Accelerator Laboratory, Center for Particle Astrophysics, Batavia, IL 60510 USA*

<sup>6</sup>*Département de Physique, Université de Montréal, Montréal, Québec H3C 3J7, Canada*

<sup>7</sup>*Department of Physics, Harvard University, Cambridge, MA 02138 USA*

<sup>8</sup>*Kavli Institute for Particle Astrophysics and Cosmology, Menlo Park, CA 94025 USA*

<sup>9</sup>*Kavli Institute for Cosmological Physics, University of Chicago, Chicago, IL 60637, USA*

November 18, 2020

This document accompanies the article titled "Effect on Dark Matter Exclusion Limits from New Silicon Photoelectric Absorption Measurements" [1], and describes the photoelectric absorption cross section data used to produce its results. The photoelectric absorption cross section data used in Ref. [1] are contained in four files:

- `pexsec_Si_nominal_keV_cm2g.txt`,
- `pexsec_Si_fitted_keV_cm2g.txt`,
- `sig1_Si_nominal_keV_eV.txt`,
- `sig1_Si_fitted_keV_eV.txt`.

In each file, the first column is the photon energy in units of keV, and the second column is the absorption data at each photon energy. The files starting with `pexsec` correspond to the photoelectric absorption cross section data ( $\sigma_{\text{p.e.}}$ ) used in the light dark matter scattering and axion-like particle absorption dark matter models. The files starting with `sig1` correspond to the real part of the complex conductivity ( $\sigma_1$ , proportional to  $\sigma_{\text{p.e.}}$ ) used in the dark photon absorption dark matter model. The absorption units are indicated by the last segment of the file name:  $\text{cm}^2/\text{g}$  for  $\sigma_{\text{p.e.}}$  and eV for  $\sigma_1$ .

The files containing `fitted` correspond to new precise measurements of the photoelectric absorption cross section described in Ref. [2]. These curves are generated by first fitting the absorption model in Ref. [3] to the measurements in Ref. [2], and then evaluating the fitted model at 50 mK. The absorption model in Ref. [3] and thus these fitted curves are valid up to a photon energy of 4 eV.

The files containing `nominal` correspond to the photoelectric absorption cross section curve using nominal, commonly used data sources. The nominal dataset is defined as the  $\sigma_{\text{p.e.}}$  data from Ref. [4] for energies  $\leq 1$  keV, Ref. [5] for energies  $> 1$  keV and  $\leq 20$  keV, and Ref. [6] for energies  $> 20$  keV. To generate the curves used in this analysis [1], the nominal data was aggregated and linearly interpolated for energies below 0.2 keV. Above 0.2 keV, the data was interpolated using an inverse cubic dependence.

The analysis in Ref. [1] compares the effect on dark matter exclusion limit between using the fitted or nominal photoelectric absorption curves. Although the fitted curve is only valid up to a photon energy of

4 eV, the photoelectric absorption is needed over a wide range of energies. Thus, for energies larger than 4 eV, previously existing data is used starting at 4.02 eV (the closest data point in the nominal dataset), interpolating in the region in between. The corresponding photoelectric absorption curves above 4.02 eV. are identical to the nominal curves.

## References

- [1] B. von Krosigk, M.J. Wilson, C. Stanford, B. Cabrera, R. Calkins, D. Jardin, N.A. Kurinsky, F. Ponce, and C.-P. Wu. Effect on Dark Matter Exclusion Limits from New Silicon Photoelectric Absorption Measurements. arXiv:2010.15874. Submitted for publication.
- [2] C. Stanford, M.J. Wilson, B. Cabrera, M. Diamond, N.A. Kurinsky, R.A. Moffatt, F. Ponce, B. von Krosigk, and B.A. Young. Photoelectric absorption cross section of silicon near the band gap from room temperature to sub-Kelvin temperature. arXiv:2010.15844. Submitted for publication.
- [3] K. Rajkanan, R. Singh, and J. Shewchun. Absorption coefficient of silicon for solar cell calculations. *Solid State Electron.*, 22:793, 1979. ISSN 0038-1101. doi: [https://doi.org/10.1016/0038-1101\(79\)90128-X](https://doi.org/10.1016/0038-1101(79)90128-X). URL <http://www.sciencedirect.com/science/article/pii/003811017990128X>.
- [4] David F. Edwards. - silicon (si)\*. In Edward D. Palik, editor, *Handbook of Optical Constants of Solids*, pages 547 – 569. Academic Press, Burlington, 1997. ISBN 978-0-12-544415-6. doi: <https://doi.org/10.1016/B978-012544415-6.50027-3>. URL <http://www.sciencedirect.com/science/article/pii/B9780125444156500273>.
- [5] B.L. Henke, E.M. Gullikson, and J.C. Davis. X-ray interactions: Photoabsorption, scattering, transmission, and reflection at  $e = 50\text{-}30,000$  eV,  $z = 1\text{-}92$ . *Atomic Data and Nuclear Data Tables*, 54(2):181 – 342, 1993. ISSN 0092-640X. doi: <https://doi.org/10.1006/adnd.1993.1013>. URL <http://www.sciencedirect.com/science/article/pii/S0092640X83710132>.
- [6] M. J. Berger, J. H. Hubbell, S. M. Seltzer, J. Chang, Coursey, R. Sukumar, D. S. Zucker, and K. Olsen. XCOM: Photon cross section database (version 1.5), 2010. URL <http://physics.nist.gov/xcom>.
